# Supplementary material for: SPARK: Multi-Vision Sensor Perception and Reasoning Benchmark for Large-scale Vision-Language Models
Source: arXiv:2408.12114 source file (2024-10-11)
Supplement: Supplementary file 1 [file Supplementary_Materials.pdf]

## Supplementary Materials of ⚡ SPARK

### Additional Question and Answer Examples

In this section, we present supplementary materials for our proposed SPARK evaluation benchmark. To be specific, we provide additional question and answer examples by evaluating four representative Large-scale Vision Language Models (LVLMs) on Multi-vision Perception and Multi-vision Reasoning tasks. We selected one model (GPT-4o) (OpenAI 2024) from a closed-source framework and the remaining three from open-source frameworks. The four representative LVLMs are:

- LLaVA-v1.5-7B (Liu et al. 2024)
- InternVL2-8B (OpenGVLab 2024)
- TroL-7B (Lee et al. 2024)
- GPT-4o (OpenAI 2024)

Multi-vision Perception task includes the following components: Existence, Counting, Position, and General Description. Multi-vision Reasoning task covers Contextual Reasoning and Sensory Reasoning. These tasks encompass six distinct multi-vision sensory categories:

- Existence
- Counting
- Position
- General Description
- Contextual Reasoning
- Sensory Reasoning

Multi-vision sensors include RGB, thermal, depth, and X-ray(XR) sensors. For clarity in the figures provided, green font indicates the correct answer, while red font denotes the incorrect answer.

### References

- Lee, B.-K.; Chung, S.; Kim, C. W.; Park, B.; and Ro, Y. M. 2024. TroL: Traversal of Layers for Large Language and Vision Models. arXiv:2406.12246.
- Liu, H.; Li, C.; Wu, Q.; and Lee, Y. J. 2024. Visual instruction tuning. *Advances in neural information processing systems*, 36.
- OpenAI. 2024. Hello GPT-4o. <https://openai.com/index/hello-gpt-4o/>.
- OpenGVLab. 2024. InternVL2: Better than the Best—Expanding Performance Boundaries of Open-Source Multimodal Models with the Progressive Scaling Strategy. <https://internvl.github.io/blog/2024-07-02-InternVL-2.0/>.

# Existence

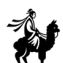

InternVL2

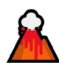

LLaVA v1.5

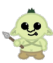

Trol

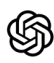

GPT-4o

RGB

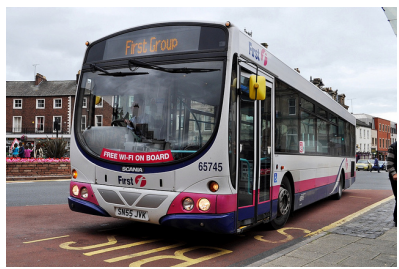

Q: Is there a bus in this image?

A: Yes

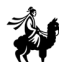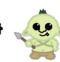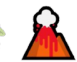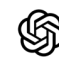

A: No

Thermal

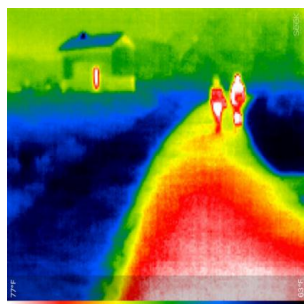

Q: Is there water visible in this image?

A: Yes

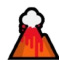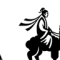

A: No

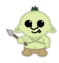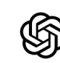

Depth

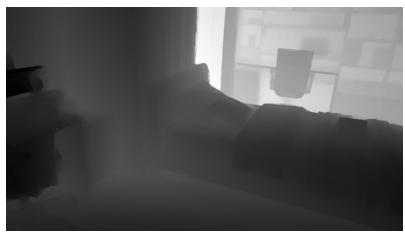

Q: Is there bed in this image?

A: Yes

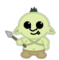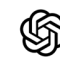

A: No

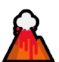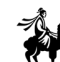

XR

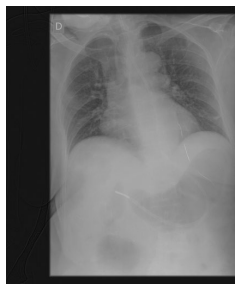

Q: Is there a ribcage in this mage?

A: Yes

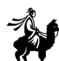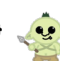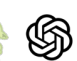

A: No

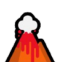

Figure 1: The comparison of sensory reasoning performance across different multi-vision sensors with respect to the representative LVLMs in the Multi-vision Perception task (Existence). Green font denotes the correct answer, while red font denotes the incorrect answer.

## Counting

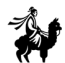

InternVL2

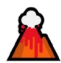

LLaVA v1.5

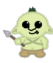

Trol

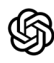

GPT-4o

**RGB**

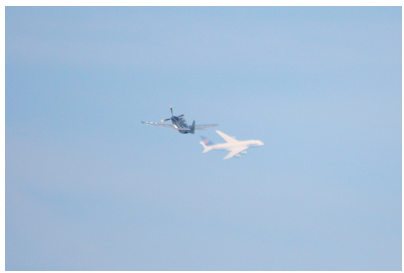

Q: Are there four aircraft in this image?

**A: Yes**

**A: No**

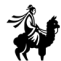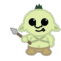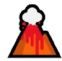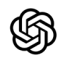

**Thermal**

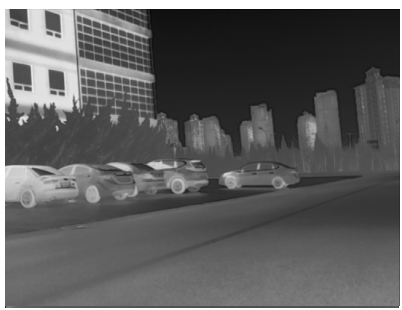

Q: Are there five cars in this image?

**A: Yes**

**A: No**

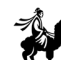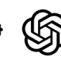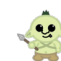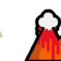

**Depth**

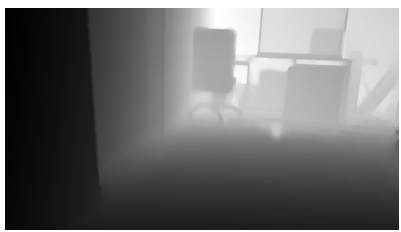

Q: Is there only one chair in this image?

**A: Yes**

**A: No**

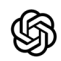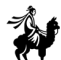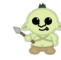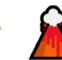

**XR**

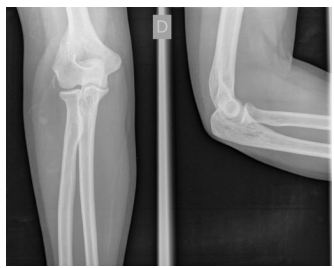

Q: Are there two legs visible in the image?

**A: Yes**

**A: No**

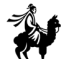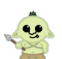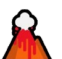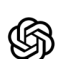

Figure 2: The comparison of sensory reasoning performance across different multi-vision sensors with respect to the representative LVLMs in the Multi-vision Perception task(Counting). Green font denotes the correct answer, while red font denotes the incorrect answer.

## Position

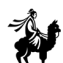

InternVL2

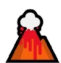

LLaVA v1.5

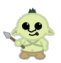

Trol

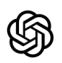

GPT-4o

RGB

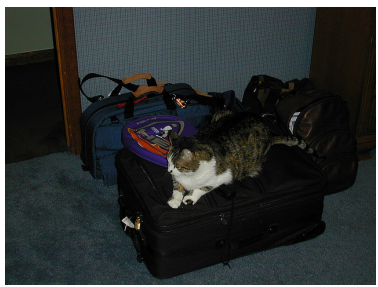

Q: Is the cat on top of the suitcase?

A: Yes

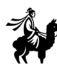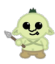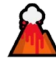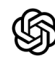

A: No

Thermal

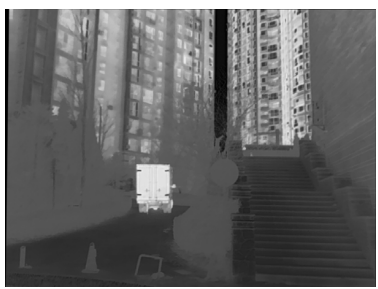

Q: Is the stairway on the right of the truck in the image?

A: Yes

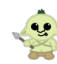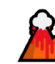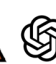

A: No

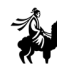

Depth

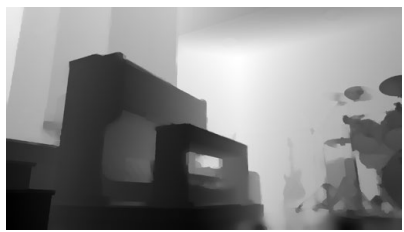

Q: Is the piano on the left the drum set in the image?

A: Yes

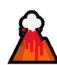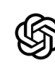

A: No

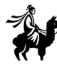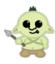

XR

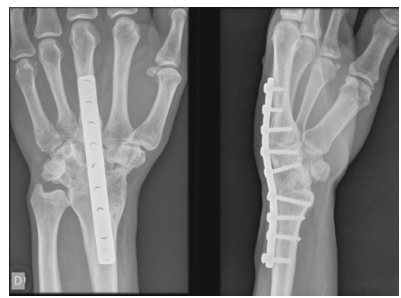

Q: Is the metal plate perpendicular to the bone?

A: Yes

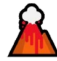

A: No

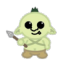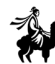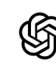

Figure 3: The comparison of sensory reasoning performance across different multi-vision sensors with respect to the representative LVLMs in the Multi-vision Perception task(Position). Green font denotes the correct answer, while red font denotes the incorrect answer.

## General Description

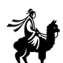

InternVL2

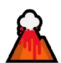

LLaVA v1.5

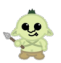

Trol

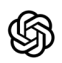

GPT-4o

**RGB**

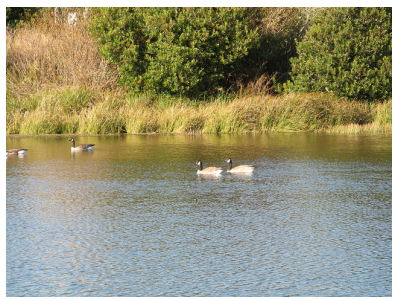

Q: Does this image depict a mountain landscape?

**A: Yes**

A: No

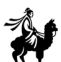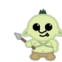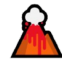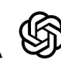

**Thermal**

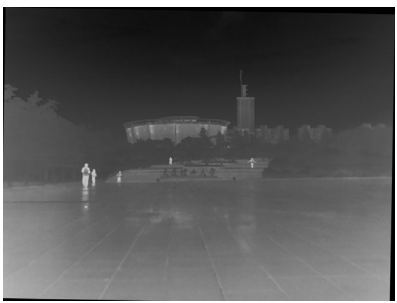

Q: Does this image depict a sports arena?

A: Yes

**A: No**

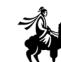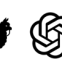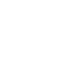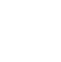

**Depth**

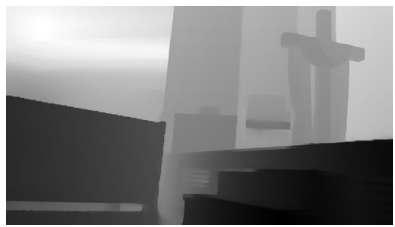

Q: Does this image describe a church?

A: Yes

**A: No**

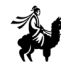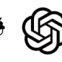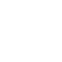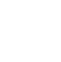

**XR**

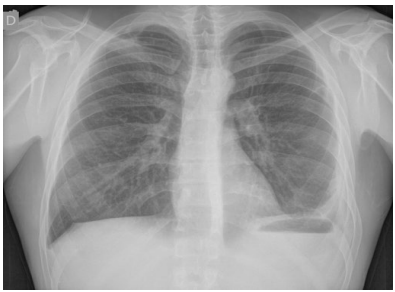

Q: Does the image show a spine?

**A: Yes**

A: No

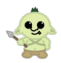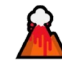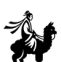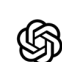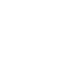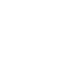

Figure 4: The comparison of sensory reasoning performance across different multi-vision sensors with respect to the recent LVLMs in the Multi-vision Perception task(General Description). Green font denotes the correct answer, while red font denotes the incorrect answer.

## Contextual Reasoning

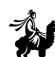 InternVL2
 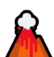 LLaVA v1.5
 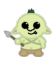 Trol
 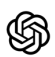 GPT-4o

|                                                                                     |                                                                                                                                                                                                                                                                                                                                                                                                                                                                                                                                                                                                                                                                   |
|-------------------------------------------------------------------------------------|-------------------------------------------------------------------------------------------------------------------------------------------------------------------------------------------------------------------------------------------------------------------------------------------------------------------------------------------------------------------------------------------------------------------------------------------------------------------------------------------------------------------------------------------------------------------------------------------------------------------------------------------------------------------|
| 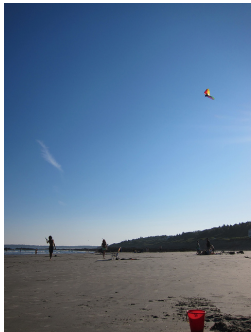   | <p><b>RGB</b></p> <p>Q: What activity are the individuals engaged in at beach?</p> <p>A: Swimming in the ocean</p> <p><b>B: Flying a kite</b> 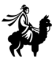 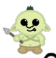 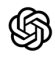</p> <p><b>C: Building a sandcastle</b> 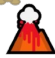</p> <p>D: Playing volleyball</p>                                                                                                |
| 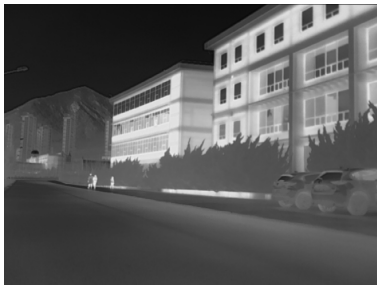   | <p><b>Thermal</b></p> <p>Q: What might the people in the image be doing in this environment?</p> <p><b>A. Shopping at a store</b> 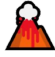</p> <p>B. Playing a sport</p> <p><b>C. Walking to a nearby building</b> 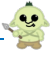 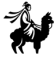 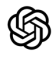</p> <p>D. Waiting for a bus</p>                                                                          |
| 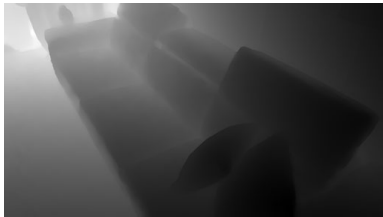 | <p><b>Depth</b></p> <p>Q: What might be the reason for the furniture in the image?</p> <p>A. To maximize storage space.</p> <p><b>B. To block sunlight from entering the room.</b> 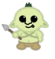</p> <p>C. To facilitate easy movement around the room</p> <p><b>D. To create a cozy and inviting living space.</b> 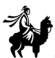 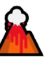 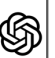</p> |
| 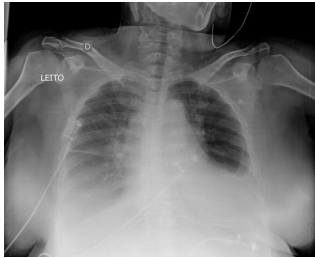 | <p><b>XR</b></p> <p>Q: What could be the reason for the prominent labeling on the image?</p> <p><b>A. Marking the age of the patient</b> 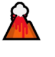</p> <p>B. Displaying the level of sedation</p> <p><b>C. Highlighting a fracture</b> 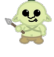</p> <p><b>D. Indicating the patient's position or orientation</b> 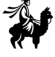 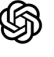</p>          |

Figure 5: The comparison of sensory reasoning performance across different multi-vision sensors with respect to the recent LVLMs in the Multi-vision Reasoning task(Contextual Reasoning). Green font denotes the correct answer, while red font denotes the incorrect answer.

## Sensory Reasoning

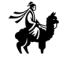

InternVL2

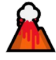

LLaVA v1.5

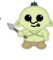

T5

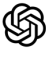

GPT-4o

**RGB**

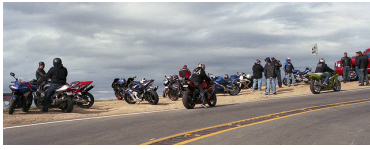

Q: What could be the likely reason for capturing this image?

- A. To advertise a new motorcycle safety gear collection.
- B. To capture a group of friends taking a leisurely ride in the countryside.

**C. To document a motorcycle gathering or event.** 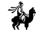 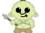 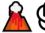

D. To promote an upcoming road construction project.

**Thermal**

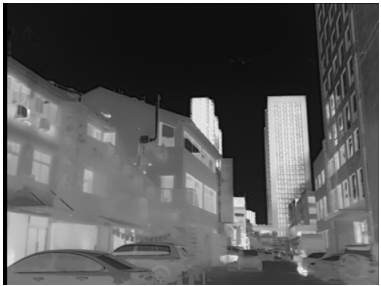

Q: What could be the likely objective of capturing this image?

A. To monitor air quality in the environment.

**B. To analyze traffic patterns in real-time.** 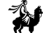 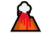

**C. To assess urban heat distribution and identify thermal anomalies.** 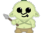 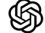

D. To evaluate the structural integrity of buildings.

**Depth**

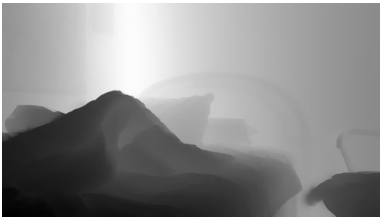

Q: What could be likely reason for capturing this image??

**A. To describe the lighting conditions.** 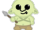

**B. To analyze the three-dimensional layout of the room and objects within it.** 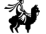 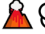 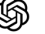

C. To assess the temperature of the objects.

D. To identify individual items on the bed.

**XR**

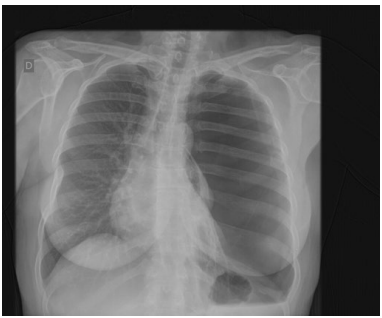

Q: What might be one purpose of capturing this medical image?

**A. To observe the size of the breasts** 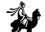

B. To measure blood alcohol levels

**C. To examine the condition of the organs** 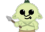 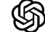

**D. To measure muscle mass** 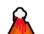

Figure 6: The comparison of sensory reasoning performance across different multi-vision sensors with respect to the recent LVLMs in the Multi-vision Reasoning task(Sensory Reasoning). Green font denotes the correct answer, while red font denotes the incorrect answer.
